# Supplementary material for: Model-independent unbinned analysis of $B \to K^*(\to K^+\pi^-)\mu^+\mu^-$: zeroes, bounds, Wilson coefficients and symmetries
Source: arXiv:2504.00949 source file (2025-07-08)

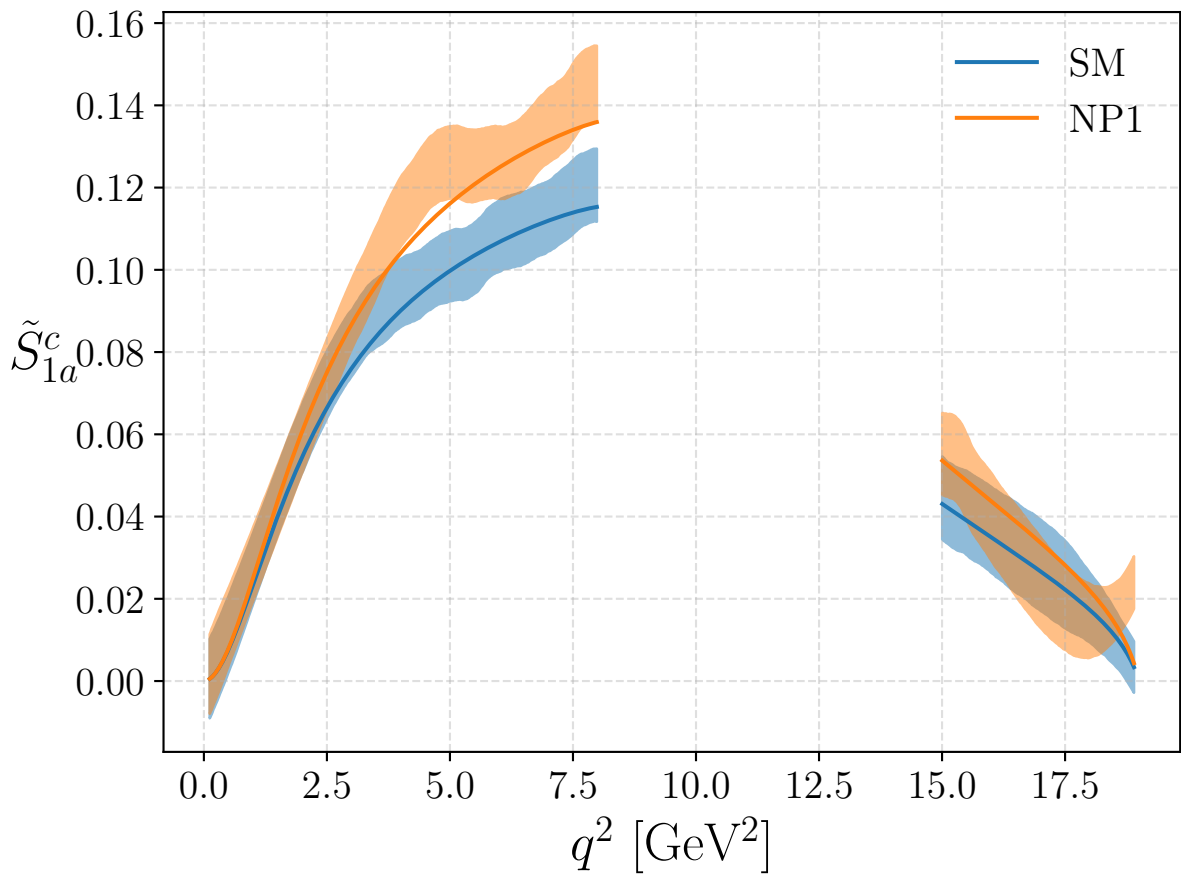

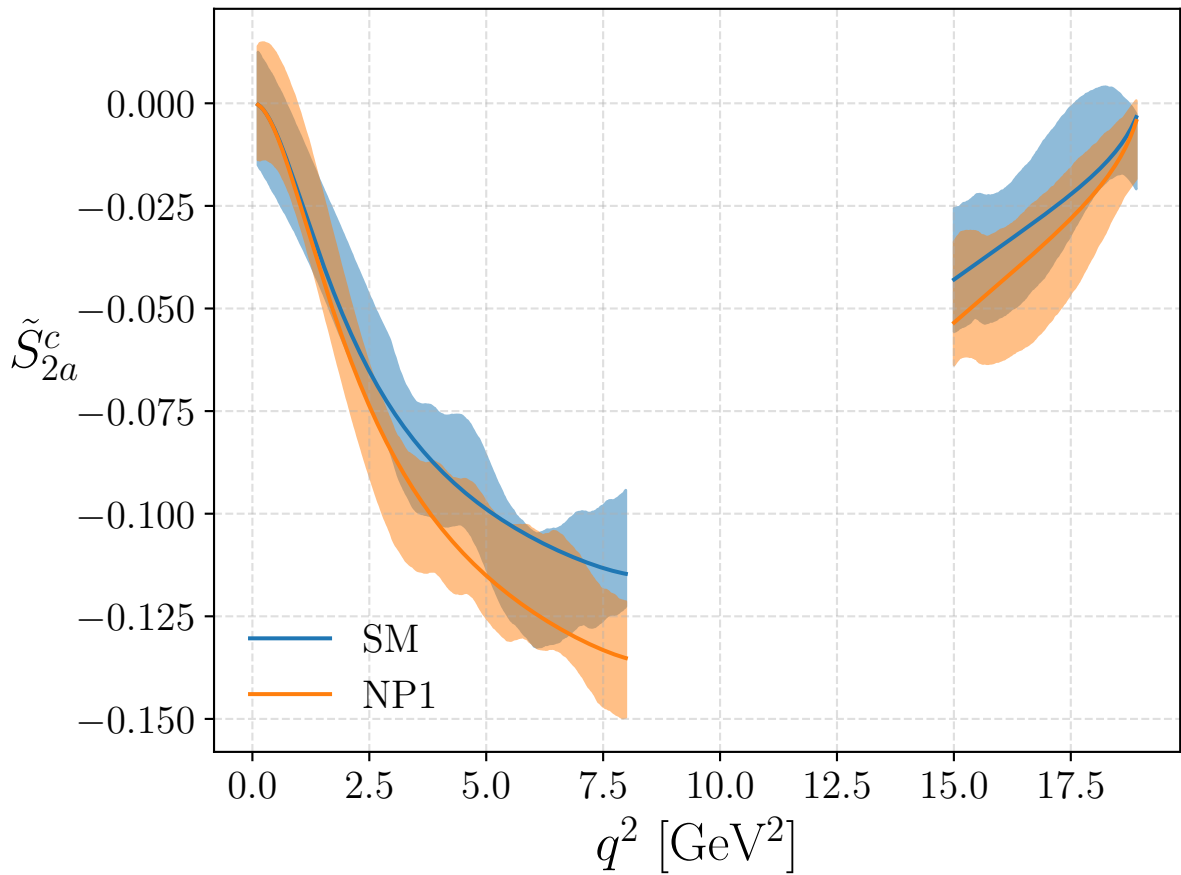

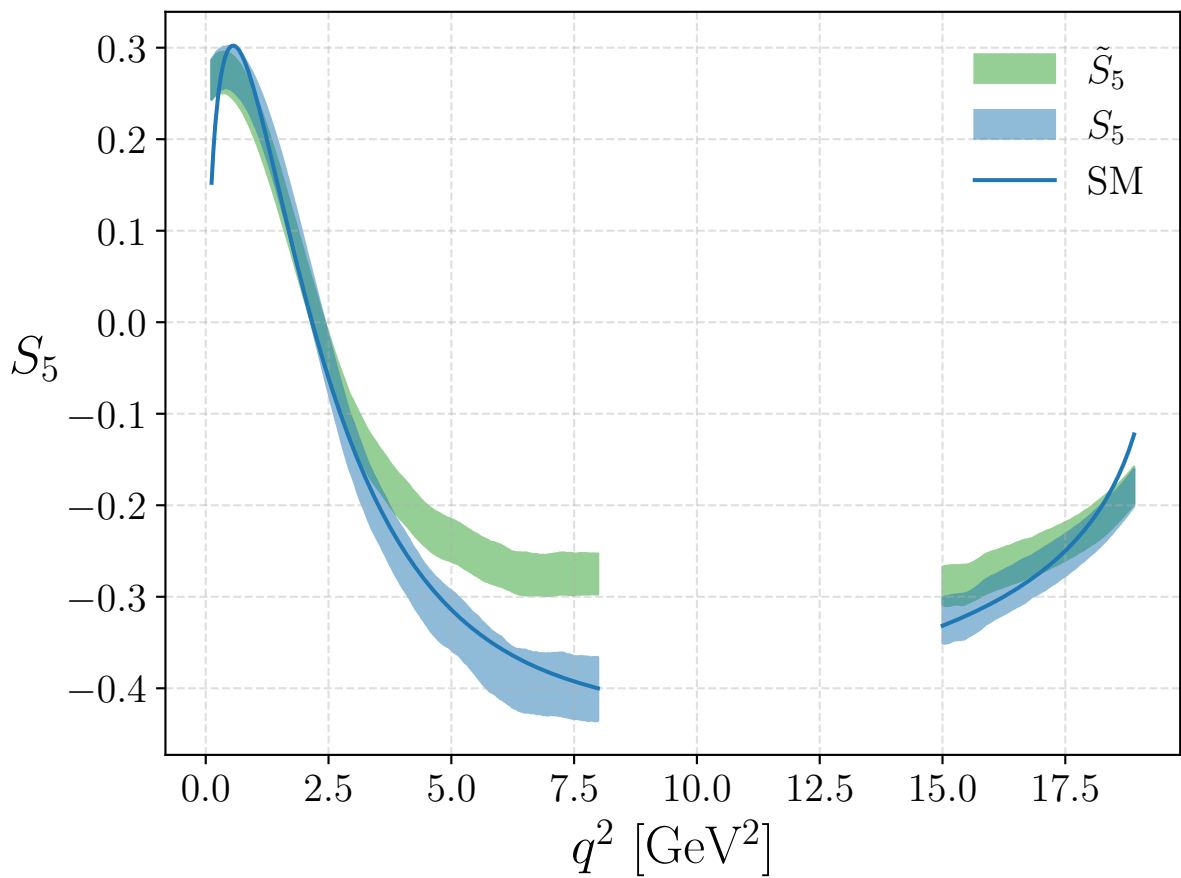

Supplement: Supplementary file 1 [file si_observables_with_swave_trim.pdf]
